# Supplementary material for: VALUE: A Multi-Task Benchmark for Video-and-Language Understanding Evaluation
Source: arXiv:2106.04632 source file (2021-08-18)
Supplement: Supplementary file 1 [file keywords.tex]

% \begin{table*}[h]
% \caption{
% Top-20 most frequent nouns and verbs used in subtitles/annotations. Character names have been filtered out from TV/VIOLIN/VLEP.
% }
% \subfloat[Subtitle
% \label{tab:keyword_sub}]{
% \tablestyle{2pt}{1.8} 
% \def\w{175pt} 

% \begin{tabular}{l|L{\w}L{\w}}
% Dataset & Nouns & Verbs\\  
% \shline
% TV & time, something, guy, way, right, man, thing, look, night, anything, god, someone, nothing, life, day, thank, kind, wait, woman, everything &
% know, go, think, want, see, need, tell, say, take, make, let, mean, come, find, give, look, talk, believe, love, feel \\
% \hline
% How2 & bit, way, kind, time, water, today, thing, lot, side, video, music, right, let, something, oil, cup, sugar, top, part, half &
% make, want, go, see, know, use, take, put, need, add, let, show, think, start, give, look, keep, cut, come, say \\
% \hline
% VIOLIN & time, something, god, look, thing, way, right, man, guy, day, night, mom, anything, thank, kind, nothing, wait, life, baby, let & 
% know, go, think, want, see, say, tell, take, need, let, come, make, mean, look, give, love, feel, talk, believe, call \\
% \hline
% VLEP & time, look, kind, something, thing, right, way, man, day, music, lot, everything, let, bit, guy, thank, food, night, place, god &
% know, go, think, see, want, need, make, take, let, say, come, love, look, mean, tell, give, try, feel, find, eat\\
% \hline
% VATEX & way, time, bit, side, look, god, job, alright, thing, kind, hand, man, today, video, day, right, lot, water, thank, something &
% go, know, see, want, make, take, think, let, put, say, come, need, keep, look, use, give, start, show, hold, love\\
% \hline
% YC2 & bit, oil, water, salt, sauce, pepper, time, kind, teaspoon, heat, pan, cup, chicken, onion, half, way, butter, garlic, side, flavor &
% add, want, make, put, use, go, take, let, see, cook, know, need, give, mix, start, cut, keep, turn, think, look\\
% \end{tabular}
% }

% \subfloat[Query/Question/Caption
% \label{tab:keyword_ann}]{
% \tablestyle{2pt}{1.8} 
% \def\w{170pt} 

% \begin{tabular}{l|L{\w}L{\w}}
% Dataset & Nouns & Verbs\\  
% \shline
% TVR/TVC & walk, hand, room, door, table, conversation, patient, man, phone, woman, apartment, head, talk, bed, front, chair, coffee, arm, tell, couch 
% & talking, walk, take, look, put, sitting, stand, turn, open, holding, sits, tell, hold, pick, asks, say, standing, give, go, looking\\
% TVQA & & \\
% How2R & man, woman, video, lady, person, car, bowl, paper, hand, ingredient, girl, food, piece, plant, water, pan, glass, guy, kitchen, chef
% & make, explain, talking, show, using, showing, making, explaining, put, add, explains, cut, shown, cooking, describes, cutting, hold, holding, use, take\\
% How2QA & video, color, man, woman, person, lady, hand, name, kind, type, bowl, food, ingredient, shirt, car, girl, item, table, boy, paper
% & used, shown, talking, using, put, wearing, added, make, holding, use, seen, cut, hold, want, mentioned, making, add, show, happen, explain\\
% VIOLIN & man, woman, shirt, suit, hair, jacket, blonde, girl, lady, brunette, dress, boy, sweater, grey, friend, room, blue, men, pink, guy
% & wearing, tell, want, asks, sitting, say, explains, talking, trying, haired, see, go, think, make, walk, take, know, holding, going, look\\
% VLEP & man, food, door, tell, room, woman, hand, patient, table, phone, shirt, walk, apartment, something, friend, vlogger, baby, girl, question, someone
% & say, tell, take, go, put, asks, look, give, start, walk, make, talk, going, leave, want, open, see, eat, turn, continue\\
% VATEX-EN-R/-C & man, woman, person, people, boy, girl, group, hand, someone, music, child, ball, men, baby, water, room, piece, front, kid, floor & playing, using, sitting, play, holding, talking, standing, showing, make, wearing, shown, dancing, riding, put, show, stand, demonstrating, throw, demonstrates, hold\\
% YC2R/YC2C & pan, oil, onion, salt, water, sauce, pepper, bowl, place, mix, pot, egg, potato, stir, chicken, mixture, slice, powder, butter, heat 
% & add, cut, mix, put, cook, chopped, remove, fry, take, chop, cover, spread, serve, stir, pour, roll, drain, flip, blend, baking\\
% \end{tabular}
% }

% \vspace{-2mm}
% \label{tab:keywords}
% \end{table*}
